# Supplementary material for: Enhancing LLM Agents for Code Generation with Possibility and Pass-rate Prioritized Experience Replay
Source: arXiv:2410.12236 source file (2025-01-11)
Supplement: Supplementary file 1 [file 6_appendix.tex]

\appendix

\section {Details for experiments in determinng hyperparameter k}
In this section, we will introduce the details of experiment in which we determine the value of hyperparameter k. As is shown in Table5, we compare the pass rates of GPT-2 in different datasets including APPS, CodeContests and Humaneval when the value of beam search k ranges from 1 to 10.
Similarly, we do experiments in GPT-neo, WrzardCoder and GPT-4-turbo as shown in Table6, Table7 and Table8. It is obvious that as the value of k increases from 1 to 3, the pass rate of code model in each datasets increase while the pass rate stays stable as the value of k surpasses 3. Therefore we decide to use k=3 as our hyperparameter. 

\begin{table*}[h!]
\centering
 % 调整行间距
\scalebox{0.84}{
\begin{tabular}{lcccccccc}
\toprule
 & \multicolumn{4}{c}{\textbf{Pass Rate (\%)}} \\
\cmidrule(lr){2-6} 
\textbf{} & \textbf{APPS Intro.} & \textbf{APPS Inter.} & \textbf{APPS comp.} & \textbf{CodeContests} & \textbf{HumanEval} \\
\midrule
\textbf{k} & & & & & & & & \\
\textbf{1} & 8.72 & 7.92 & 6.33 & 10.30 & 11.30  \\
\textbf{2} & 9.79 & 8.50 & 7.10 & 11.00 & 11.50 \\
\textbf{3} & 10.98 & 9.30 & 7.90 & 11.50 & 12.00  \\
\textbf{4} & 11.01 & 9.00 & 7.70 & 11.20 & 11.80 \\
\textbf{5} & 11.23 & 9.20 & 7.50 & 11.30 & 11.90  \\
\textbf{6} & 11.40 & 9.10 & 7.40 & 11.10 & 11.70 \\
\textbf{7} & 11.52 & 9.00 & 7.30 & 11.00 & 11.60 \\
\textbf{8} & 11.23 & 8.90 & 7.20 & 10.90 & 11.50 \\
\textbf{9} & 11.52 & 9.10 & 7.50 & 11.20 & 11.80 \\
\textbf{10} & 11.83 & 9.30 & 7.70 & 11.50 & 12.00 \\
\bottomrule
\end{tabular}}
\caption{The pass rate of GPT2 using beam search in different k}
\label{table:accuracy}
\end{table*}

\vspace{6cm}

\begin{table*}[h!]
\centering
 % 调整行间距
\scalebox{0.84}{
\begin{tabular}{lcccccccc}
\toprule
 & \multicolumn{4}{c}{\textbf{Pass Rate (\%)}} \\
\cmidrule(lr){2-6} 
\textbf{} & \textbf{APPS Intro.} & \textbf{APPS Inter.} & \textbf{APPS comp.} & \textbf{CodeContests} & \textbf{HumanEval} \\
\midrule
\textbf{k} & & & & & & & & \\
\textbf{1} & 10.72 & 9.92 & 8.33 & 13.30 & 14.30  \\
\textbf{2} & 11.79 & 10.50 & 9.10 & 15.00 & 16.50 \\
\textbf{3} & 11.98 & 11.30 & 9.90 & 15.59 & 17.93  \\
\textbf{4} & 12.02 & 11.00 & 10.70 & 15.21 & 17.81 \\
\textbf{5} & 12.28 & 11.20 & 9.94 & 15.30 & 17.92  \\
\textbf{6} & 12.95 & 10.92 & 10.22 & 14.50 & 18.02 \\
\textbf{7} & 12.82 & 11.00 & 10.15 & 15.20 & 17.23 \\
\textbf{8} & 12.57 & 10.90 & 10.53 & 15.92 & 17.52 \\
\textbf{9} & 12.59 & 11.10 & 9.78 & 16.24 & 16.92 \\
\textbf{10} & 12.53 & 10.82 & 10.23 & 15.51 & 17.00 \\
\bottomrule
\end{tabular}}
\caption{The pass rate of GPT-Neo using beam search in different k}
\label{table:accuracy}
\end{table*}

\begin{table*}[h!]
\centering
 % 调整行间距
\scalebox{0.84}{
\begin{tabular}{lcccccccc}
\toprule
 & \multicolumn{4}{c}{\textbf{Pass Rate (\%)}} \\
\cmidrule(lr){2-6} 
\textbf{} & \textbf{APPS Intro.} & \textbf{APPS Inter.} & \textbf{APPS comp.} & \textbf{CodeContests} & \textbf{HumanEval} \\
\midrule
\textbf{k} & & & & & & & & \\
\textbf{1} & 56.39 & 55.22 & 52.02 & 60.29 & 59.23  \\
\textbf{2} & 57.29 & 49.00 & 45.10 & 58.00 & 57.50 \\
\textbf{3} & 60.92 & 53.00 & 50.90 & 60.50 & 59.00  \\
\textbf{4} & 60.01 & 51.00 & 49.70 & 59.20 & 58.80 \\
\textbf{5} & 60.23 & 52.00 & 47.50 & 59.30 & 58.90  \\
\textbf{6} & 59.40 & 50.90 & 47.40 & 59.10 & 58.70 \\
\textbf{7} & 60.52 & 51.00 & 47.30 & 59.00 & 58.60 \\
\textbf{8} & 60.23 & 50.90 & 47.20 & 58.90 & 58.50 \\
\textbf{9} & 61.52 & 51.10 & 47.50 & 59.20 & 58.80 \\
\textbf{10} & 60.83 & 51.30 & 47.70 & 59.50 & 59.00 \\
\bottomrule
\end{tabular}}
\caption{The pass rate of WizardCoder using beam search in different k}
\label{table:accuracy}
\end{table*}

\vspace{6cm}
\begin{table*}[h!]
\centering
 % 调整行间距
\scalebox{0.84}{
\begin{tabular}{lcccccccc}
\toprule
 & \multicolumn{4}{c}{\textbf{Pass Rate (\%)}} \\
\cmidrule(lr){2-6} 
\textbf{} & \textbf{APPS Intro.} & \textbf{APPS Inter.} & \textbf{APPS comp.} & \textbf{CodeContests} & \textbf{HumanEval} \\
\midrule
\textbf{k} & & & & & & & & \\
\textbf{1} & 79.24& 76.22 & 70.02 & 86.29 & 70.23  \\
\textbf{2} & 80.93 & 78.00 & 72.10 & 88.00 & 72.50 \\
\textbf{3} & 82.83 & 78.00 & 72.90 & 89.99 & 74.00  \\
\textbf{4} & 82.01 & 78.00 & 71.70 & 90.01 & 73.82 \\
\textbf{5} & 82.23 & 77.21 & 72.50 & 89.34 & 74.21  \\
\textbf{6} & 82.40 & 79.90 & 72.40 & 89.10 & 73.76 \\
\textbf{7} & 82.52 & 78.04 & 71.30 & 89.00 & 74.64 \\
\textbf{8} & 82.23 & 78.92 & 72.20 & 88.90 & 74.55 \\
\textbf{9} & 83.52 & 77.15 & 72.50 & 89.20 & 73.82 \\
\textbf{10} & 83.83 & 78.34 & 73.70 & 89.50 & 74.00 \\
\bottomrule
\end{tabular}}
\caption{The pass rate of GPT-4-turbo using beam search in different k}
\label{table:accuracy}
\end{table*}

\clearpage
\section {A small experiment about $\alpha$}
In this section, we perform a small experiment to discuss about the influence of the value of $\alpha$ in the PPER phase. However, the optimal value varies across different models and datasets. As is shown from Table9-Table12, the most appropriate value of $\alpha$ ranges in different model and datasets. And figure2-figure5 shows more details about the results.

\begin{table*}[h!]
\centering
 % 调整行间距
\scalebox{0.84}{
\begin{tabular}{lcccccccc}
\toprule
 & \multicolumn{4}{c}{\textbf{Pass Rate (\%)}} \\
\cmidrule(lr){2-6} 
\textbf{} & \textbf{APPS Intro.} & \textbf{APPS Inter.} & \textbf{APPS comp.} & \textbf{CodeContests} & \textbf{HumanEval} \\
\midrule
\textbf{$\alpha$} & & & & & & & & \\
\textbf{0} & 18.57 & 22.11 & 20.05 & 22.82 & 24.45  \\
\textbf{0.05} & 21.60 & 21.79 & 24.44 & 24.04 & 24.23 \\
\textbf{0.1} & 21.58 & 21.81 & 21.28 & 23.22 & 26.84 \\
\textbf{0.15} & 20.07 & 24.29 & 25.23 & 23.42 & 27.13 \\
\textbf{0.2} & 20.56 & 21.67 & 24.33 & 25.08 & 24.40  \\
\textbf{0.25} & 19.83 & 22.82 & 24.36 & 25.19 & 27.76 \\
\textbf{0.3} & 20.00 & 22.03 & 23.59 & 27.35 & 28.94 \\
\textbf{0.35} & 20.35 & 22.40 & 25.14 & 27.91 & 29.42 \\
\textbf{0.4} & 21.34 & 23.65 & 25.12 & 27.93 & 29.12  \\
\textbf{0.45} & 23.11 & 25.19 & 26.51 & 27.90 & 30.65 \\
\textbf{0.5} & 21.18 & 21.18 & 25.24 & 24.12 & 27.76 \\
\textbf{0.55} & 20.57 & 22.10 & 25.80 & 24.70 & 26.87 \\
\textbf{0.6} & 21.42 & 24.52 & 26.58 & 28.40 & 27.21 \\
\textbf{0.65} & 21.64 & 22.93 & 27.32 & 27.11 & 31.52 \\
\textbf{0.7} & 21.00 & 22.90 & 26.27 & 26.73 & 31.57 \\
\textbf{0.75} & 19.71 & 22.01 & 23.20 & 26.98 & 27.64 \\
\textbf{0.8} & 21.07 & 23.27 & 23.59 & 26.38 & 29.46 \\
\textbf{0.85} & 20.14 & 23.43 & 24.30 & 26.86 & 30.01 \\
\textbf{0.9} & 20.90 & 22.99 & 26.03 & 28.22 & 29.81 \\
\textbf{0.95} & 21.31 & 23.36 & 25.36 & 27.90 & 30.49 \\
\textbf{1.0} & 20.07 & 24.29 & 25.23 & 23.42 & 27.13 \\
\bottomrule
\end{tabular}}
\caption{The pass rate of GPT-2-Wizard using BTP in different $\alpha$}
\label{table:accuracy}
\end{table*}

\vspace{6cm}
\begin{table*}[h!]
\centering
 % 调整行间距
\scalebox{0.84}{
\begin{tabular}{lcccccccc}
\toprule
 & \multicolumn{4}{c}{\textbf{Pass Rate (\%)}} \\
\cmidrule(lr){2-6} 
\textbf{} & \textbf{APPS Intro.} & \textbf{APPS Inter.} & \textbf{APPS comp.} & \textbf{CodeContests} & \textbf{HumanEval} \\
\midrule
\textbf{$\alpha$} & & & & & & & & \\
\textbf{0} & 18.68 & 22.63 & 22.20 & 26.04 & 25.83  \\
\textbf{0.05} & 20.21 & 23.27 & 22.78 & 27.09 & 26.18 \\
\textbf{0.1} & 21.22 & 24.72 & 23.34 & 28.75 & 28.49 \\
\textbf{0.15} & 21.98 & 24.48 & 23.51 & 27.88 & 28.32 \\
\textbf{0.2} & 22.09 & 25.21 & 23.69 & 28.11 & 28.45  \\
\textbf{0.25} & 19.83 & 22.82 & 24.36 & 25.19 & 27.76 \\
\textbf{0.3} & 21.89 & 23.74 & 25.10 & 28.45 & 28.98 \\
\textbf{0.35} & 20.99 & 23.40 & 25.25 & 27.71 & 29.02 \\
\textbf{0.4} & 22.38 & 23.80 & 24.96 & 28.09 & 30.51  \\
\textbf{0.45} & 23.19 & 25.04 & 26.52 & 29.35 & 31.42 \\
\textbf{0.5} & 21.35 & 22.94 & 24.81 & 26.91 & 28.67 \\
\textbf{0.55} & 20.57 & 23.36 & 25.80 & 24.70 & 26.87 \\
\textbf{0.6} & 21.91 & 24.23 & 25.98 & 29.38 & 30.08 \\
\textbf{0.65} & 22.64 & 23.64 & 26.32 & 28.77 & 31.16 \\
\textbf{0.7} & 21.11 & 22.74 & 26.11 & 27.25 & 29.59 \\
\textbf{0.75} & 20.45 & 23.16 & 23.71 & 26.80 & 28.74 \\
\textbf{0.8} & 21.67 & 23.55 & 24.87 & 27.12 & 29.78 \\
\textbf{0.85} & 20.54 & 23.26 & 24.23 & 26.41 & 29.91 \\
\textbf{0.9} & 22.12 & 23.84 & 26.12 & 28.54 & 30.14 \\
\textbf{0.95} & 20.87 & 23.43 & 24.91 & 27.37 & 29.08 \\
\textbf{1.0} & 22.00 & 24.63 & 25.51 & 28.16 & 30.33 \\
\bottomrule
\end{tabular}}
\caption{The pass rate of GPT2-Llama using BTP in different $\alpha$}
\label{table:accuracy}
\end{table*}

\begin{table*}[h!]
\centering
 % 调整行间距
\scalebox{0.84}{
\begin{tabular}{lcccccccc}
\toprule
 & \multicolumn{4}{c}{\textbf{Pass Rate (\%)}} \\
\cmidrule(lr){2-6} 
\textbf{} & \textbf{APPS Intro.} & \textbf{APPS Inter.} & \textbf{APPS comp.} & \textbf{CodeContests} & \textbf{HumanEval} \\
\midrule
\textbf{$\alpha$} & & & & & & & & \\
\textbf{0} & 38.69 & 43.24 & 46.15 & 48.77 & 49.85  \\
\textbf{0.05} & 39.00 & 42.62 & 46.69 & 50.88 & 49.73 \\
\textbf{0.1} & 40.18 & 44.80 & 48.04 & 49.63 & 52.70 \\
\textbf{0.15} & 40.00 & 44.58 & 47.83 & 50.73 & 51.68 \\
\textbf{0.2} & 41.67 & 46.50 & 48.95 & 50.63 & 52.04  \\
\textbf{0.25} & 38.69 & 43.69 & 46.28 & 49.71 & 50.58 \\
\textbf{0.3} & 40.30 & 44.75 & 48.13 & 51.42 & 52.87 \\
\textbf{0.35} & 39.12 & 44.62 & 48.21 & 51.20 & 53.34 \\
\textbf{0.4} & 41.08 & 45.03 & 48.41 & 50.91 & 54.14  \\
\textbf{0.45} & 42.18 & 46.39 & 49.85 & 52.31 & 54.81 \\
\textbf{0.5} & 40.46 & 43.88 & 47.23 & 49.41 & 51.98 \\
\textbf{0.55} & 39.61 & 44.78 & 49.15 & 47.20 & 50.06 \\
\textbf{0.6} & 41.24 & 45.32 & 48.16 & 52.71 & 53.08 \\
\textbf{0.65} & 42.45 & 44.65 & 49.04 & 52.25 & 54.38 \\
\textbf{0.7} & 40.51 & 43.85 & 49.01 & 50.76 & 52.87 \\
\textbf{0.75} & 39.90 & 44.55 & 46.86 & 50.18 & 52.44 \\
\textbf{0.8} & 41.76 & 45.64 & 47.92 & 50.67 & 53.38 \\
\textbf{0.85} & 40.39 & 45.27 & 47.52 & 50.05 & 53.27 \\
\textbf{0.9} & 42.32 & 45.95 & 49.69 & 51.64 & 53.82 \\
\textbf{0.95} & 40.94 & 45.58 & 48.88 & 50.76 & 52.70 \\
\textbf{1.0} & 42.31 & 46.59 & 49.69 & 51.64 & 53.82 \\
\bottomrule
\end{tabular}}
\caption{The pass rate of GPT2-GPT3.5 using BTP in different $\alpha$}
\label{table:accuracy_third_set}
\end{table*}

\begin{table*}[h!]
\centering
 % 调整行间距
\scalebox{0.84}{
\begin{tabular}{lcccccccc}
\toprule
 & \multicolumn{4}{c}{\textbf{Pass Rate (\%)}} \\
\cmidrule(lr){2-6} 
\textbf{} & \textbf{APPS Intro.} & \textbf{APPS Inter.} & \textbf{APPS comp.} & \textbf{CodeContests} & \textbf{HumanEval} \\
\midrule
\textbf{$\alpha$} & & & & & & & & \\
\textbf{0} & 48.69 & 53.24 & 56.15 & 58.77 & 59.85  \\
\textbf{0.05} & 49.00 & 52.62 & 56.69 & 60.88 & 59.73 \\
\textbf{0.1} & 50.18 & 54.80 & 58.04 & 59.63 & 62.70 \\
\textbf{0.15} & 50.00 & 54.58 & 57.83 & 60.73 & 61.68 \\
\textbf{0.2} & 51.67 & 56.50 & 58.95 & 60.63 & 62.04  \\
\textbf{0.25} & 48.69 & 53.69 & 56.28 & 59.71 & 60.58 \\
\textbf{0.3} & 50.30 & 54.75 & 58.13 & 61.42 & 62.87 \\
\textbf{0.35} & 49.12 & 54.62 & 58.21 & 61.20 & 63.34 \\
\textbf{0.4} & 51.08 & 55.03 & 58.41 & 60.91 & 64.14  \\
\textbf{0.45} & 52.18 & 56.39 & 59.85 & 62.31 & 64.81 \\
\textbf{0.5} & 50.46 & 53.88 & 57.23 & 59.41 & 61.98 \\
\textbf{0.55} & 49.61 & 54.78 & 59.15 & 57.20 & 60.06 \\
\textbf{0.6} & 51.24 & 55.32 & 58.16 & 62.71 & 63.08 \\
\textbf{0.65} & 52.45 & 54.65 & 59.04 & 62.25 & 64.38 \\
\textbf{0.7} & 50.51 & 53.85 & 59.01 & 60.76 & 62.87 \\
\textbf{0.75} & 49.90 & 54.55 & 56.86 & 60.18 & 62.44 \\
\textbf{0.8} & 51.76 & 55.64 & 57.92 & 60.67 & 63.38 \\
\textbf{0.85} & 50.39 & 55.27 & 57.52 & 60.05 & 63.27 \\
\textbf{0.9} & 52.32 & 55.95 & 59.69 & 61.64 & 63.82 \\
\textbf{0.95} & 50.94 & 55.58 & 58.88 & 60.76 & 62.70 \\
\textbf{1.0} & 52.31 & 56.59 & 59.69 & 61.64 & 63.82 \\
\bottomrule
\end{tabular}}
\caption{The pass rate of GPT2-GPT4 using BTP in different $\alpha$}
\label{table:accuracy_third_set}
\end{table*}
\clearpage
\begin{figure}[htbp]
    \centering
    \includegraphics[width=\linewidth]{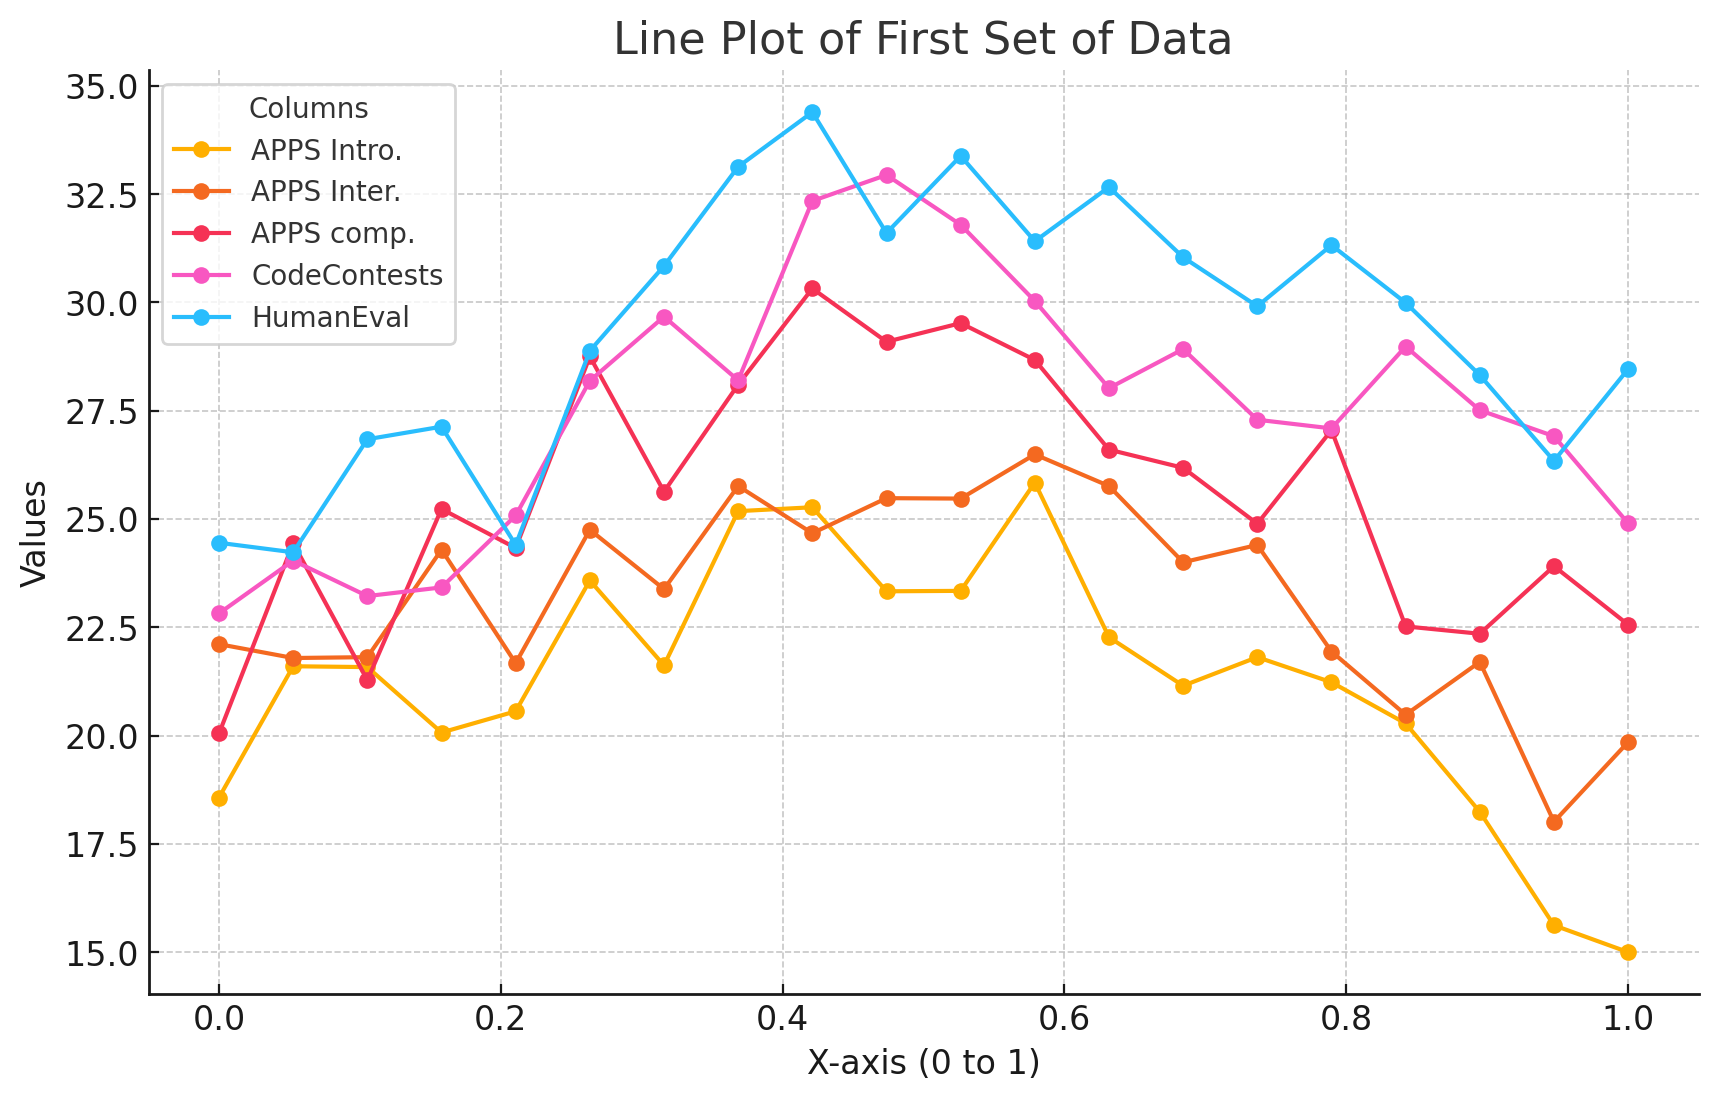}
    \caption{The pass rate of GPT2-Wizard using BTP in different $\alpha$}
    \label{fig:example}
\end{figure}
\begin{figure}[htbp]
    \centering
    \includegraphics[width=\linewidth]{content/figs/output (1).png}
    \caption{The pass rate of GPT2-Llama using BTP in different $\alpha$}
    \label{fig:example}
\end{figure}
\begin{figure}[htbp]
    \centering
    \includegraphics[width=\linewidth]{content/figs/output (2).png}
    \caption{The pass rate of GPT2-GPT3.5 using BTP in different $\alpha$}
    \label{fig:example}
\end{figure}
\begin{figure}[htbp]
    \centering
    \includegraphics[width=\linewidth]{content/figs/output (3).png}
    \caption{The pass rate of GPT2-GPT4 using BTP in different $\alpha$}
    \label{fig:example}
\end{figure}
\clearpage

\section {Details for all experiments results}
In this section, we show all experiments results including all datasets and all code models. Table13 shows better code models sample programs when tasks from CodeContests are sent. Similarly Table14-Table17 shows tasks from different datasets.

\begin{table*}[!htb]
\centering
 % 调整行间距
\scalebox{0.84}{
\begin{tabular}{lcccccccc}
\toprule
 & \multicolumn{4}{c}{\textbf{Pass Rate (\%)}} & \multicolumn{4}{c}{\textbf{Accuracy rate(\%)}} \\
\cmidrule(lr){2-5} \cmidrule(lr){6-9}
\textbf{} & \textbf{APPS Intro.} & \textbf{APPS Inter.} & \textbf{APPS comp.} & \textbf{APPS mixed} & \textbf{APPS Intro.} & \textbf{APPS Inter.} & \textbf{APPS comp.} & \textbf{APPS mixed} \\
\midrule
\textbf{CodeContests GPT-2} & & & & & & & & \\
\textbf{GPT-2} & 13.54 & 10.24 & 4.04 & 7.79 & 5.11 & 3.15 & 1.34 & 2.74 \\
\textbf{GPT-2-GPT4} & 53.92 & 41.97 & 38.41 & 39.6 & 24.76 & 19.22 & 14.5 & 20.45 \\
\textbf{GPT-2-GPT3.5} & 39.78 & 39.83 & 30.18 & 32.02 & 19.52 & 15.21 & 12.28 & 16.3 \\
\textbf{GPT-2-Llama} & 32.32 & 30.17 & 23.55 & 25.97 & 15.15 & 10.91 & 8.1 & 10.85 \\
\textbf{GPT-2-Wizard} & 36.74 & 27.7 & 22.85 & 25.73 & 13.27 & 9.27 & 5.83 & 9.58 \\
\midrule
\textbf{CodeContests GPT-Neo} & & & & & & & & \\
\textbf{GPT-Neo} & 14.45 & 10.76 & 5.8 & 5.4 & 7.05 & 2.04 & 2.05 & 3.24 \\
\textbf{GPT-Neo-GPT4} & 47.61 & 49.24 & 38.02 & 40.89 & 28.96 & 25.39 & 18.8 & 19.97 \\
\textbf{GPT-Neo-GPT3.5} & 42.9 & 31.88 & 28.81 & 31.01 & 16.15 & 10.36 & 4.84 & 9.07 \\
\textbf{GPT-Neo-Llama} & 40.81 & 31.39 & 24.33 & 28.82 & 13.34 & 11.05 & 3.74 & 7.53 \\
\textbf{GPT-Neo-Wizard} & 36.6 & 30.55 & 25.71 & 28.29 & 11.8 & 8.7 & 2.37 & 5.84 \\
\bottomrule
\end{tabular}}
\caption{Result of "Better models help fine-tune normal models" experiment. On the top and bottom of the table, we show the performance of GPT-2 and GPT-Neo, and how they perform after they are fine-tuned by programs sampled by better models including GPT-4-turbo, GPT-3.5-turbo, CodeLlama-34B, WizardCoder-34B}
\label{table:accuracy}
\end{table*}

\begin{table*}[!htb]
\centering
 % 调整行间距
\scalebox{0.84}{
\begin{tabular}{lcccccccc}
\toprule
 & \multicolumn{4}{c}{\textbf{Pass Rate (\%)}} & \multicolumn{4}{c}{\textbf{Accuracy rate(\%)}} \\
\cmidrule(lr){2-5} \cmidrule(lr){6-9}
\textbf{} & \textbf{APPS Intro.} & \textbf{APPS Inter.} & \textbf{APPS comp.} & \textbf{APPS mixed} & \textbf{APPS Intro.} & \textbf{APPS Inter.} & \textbf{APPS comp.} & \textbf{APPS mixed} \\
\midrule
\textbf{HumanEval GPT-2} & & & & & & & & \\
\textbf{GPT-2} & 13.54 & 10.24 & 4.04 & 7.79 & 5.11 & 3.15 & 1.34 & 2.74 \\
\textbf{GPT-2-GPT4} & 53.92 & 41.97 & 38.41 & 39.6 & 24.76 & 19.22 & 14.5 & 20.45 \\
\textbf{GPT-2-GPT3.5} & 39.78 & 39.83 & 30.18 & 32.02 & 19.52 & 15.21 & 12.28 & 16.3 \\
\textbf{GPT-2-Llama} & 32.32 & 30.17 & 23.55 & 25.97 & 15.15 & 10.91 & 8.1 & 10.85 \\
\textbf{GPT-2-Wizard} & 36.74 & 27.7 & 22.85 & 25.73 & 13.27 & 9.27 & 5.83 & 9.58 \\
\midrule
\textbf{HumanEval GPT-Neo} & & & & & & & & \\
\textbf{GPT-Neo} & 14.45 & 10.76 & 5.8 & 5.4 & 7.05 & 2.04 & 2.05 & 3.24 \\
\textbf{GPT-Neo-GPT4} & 47.61 & 49.24 & 38.02 & 40.89 & 28.96 & 25.39 & 18.8 & 19.97 \\
\textbf{GPT-Neo-GPT3.5} & 42.9 & 31.88 & 28.81 & 31.01 & 16.15 & 10.36 & 4.84 & 9.07 \\
\textbf{GPT-Neo-Llama} & 40.81 & 31.39 & 24.33 & 28.82 & 13.34 & 11.05 & 3.74 & 7.53 \\
\textbf{GPT-Neo-Wizard} & 36.6 & 30.55 & 25.71 & 28.29 & 11.8 & 8.7 & 2.37 & 5.84 \\
\bottomrule
\end{tabular}}
\caption{Result of "Better models help fine-tune normal models" experiment. On the top and bottom of the table, we show the performance of GPT-2 and GPT-Neo, and how they perform after they are fine-tuned by programs sampled by better models including GPT-4-turbo, GPT-3.5-turbo, CodeLlama-34B, WizardCoder-34B}
\label{table:accuracy}
\end{table*}

\begin{table*}[!htb]
\centering
 % 调整行间距
\scalebox{0.84}{
\begin{tabular}{lcccccccc}
\toprule
 & \multicolumn{2}{c}{\textbf{Pass Rate (\%)}} & \multicolumn{2}{c}{\textbf{Accuracy rate(\%)}} \\
\cmidrule(lr){2-3} \cmidrule(lr){4-5}
\textbf{} & \textbf{CodeContests} & \textbf{HumanEval} & \textbf{CodeContests} & \textbf{HumanEval} \\
\midrule
\textbf{APPS GPT-2} & & & & & & & & \\
\textbf{GPT-2} & 13.0 & 10.21  & 5.57 & 3.18  \\
\textbf{GPT-2-GPT4} & 55.57 & 39.74  & 23.27 & 17.77  \\
\textbf{GPT-2-GPT3.5} & 42.18 & 35.88  & 21.07 & 16.7  \\
\textbf{GPT-2-Llama} & 35.51 & 30.45  & 16.66 & 11.21  \\
\textbf{GPT-2-Wizard} & 38.29 & 28.39  & 12.78 & 8.96 \\
\midrule
\textbf{APPS GPT-Neo} & & & & & & & & \\
\textbf{GPT-Neo} & 13.06 & 11.17 & 6.9 & 2.19 \\
\textbf{GPT-Neo-GPT4} & 45.26 & 53.74  & 30.14 & 23.92 \\
\textbf{GPT-Neo-GPT3.5} & 42.58 & 29.31  & 16.35 & 9.82 \\
\textbf{GPT-Neo-Llama} & 44.72 & 28.79 & 14.14 & 11.55 \\
\textbf{GPT-Neo-Wizard} & 34.13 & 29.79& 12.66 & 9.52 \\
\bottomrule
\end{tabular}}
\caption{Result of "Better models help fine-tune normal models" experiment. On the top and bottom of the table, we show the performance of GPT-2 and GPT-Neo, and how they perform after they are fine-tuned by programs sampled by better models including GPT-4-turbo, GPT-3.5-turbo, CodeLlama-34B, WizardCoder-34B}
\label{table:accuracy}
\end{table*}

\begin{table*}[!htb]
\centering
 % 调整行间距
\scalebox{0.84}{
\begin{tabular}{lcccccccc}
\toprule
 & \multicolumn{2}{c}{\textbf{Pass Rate (\%)}} & \multicolumn{2}{c}{\textbf{Accuracy rate(\%)}} \\
\cmidrule(lr){2-3} \cmidrule(lr){4-5}
\textbf{} & \textbf{CodeContests} & \textbf{HumanEval} & \textbf{CodeContests} & \textbf{HumanEval} \\
\midrule
\textbf{CodeContests GPT-2} & & & & & & & & \\
\textbf{GPT-2} & 14.71 & 9.88  & 5.3 & 3.28  \\
\textbf{GPT-2-GPT4} & 48.64 & 46.16  & 25.19 & 20.35  \\
\textbf{GPT-2-GPT3.5} & 35.96 & 41.51  & 19.62 & 14.85  \\
\textbf{GPT-2-Llama} & 32.99 & 30.36  & 15.5 & 10.95  \\
\textbf{GPT-2-Wizard} & 34.85 & 25.39  & 12.37 & 9.88 \\
\midrule
\textbf{CodeContests GPT-Neo} & & & & & & & & \\
\textbf{GPT-Neo} & 15.71 & 10.5& 7.37 & 1.97 \\
\textbf{GPT-Neo-GPT4} & 44.61 & 48.63  & 29.19 & 24.75 \\
\textbf{GPT-Neo-GPT3.5} & 43.21 & 33.46  & 16.2& 10.29 \\
\textbf{GPT-Neo-Llama} & 38.95 & 28.78 & 14.63 & 10.23\\
\textbf{GPT-Neo-Wizard} & 37.19 & 30.09& 11.81 & 8.28\\
\bottomrule
\end{tabular}}
\caption{Result of "Better models help fine-tune normal models" experiment. On the top and bottom of the table, we show the performance of GPT-2 and GPT-Neo, and how they perform after they are fine-tuned by programs sampled by better models including GPT-4-turbo, GPT-3.5-turbo, CodeLlama-34B, WizardCoder-34B}
\label{table:accuracy}
\end{table*}

\begin{table*}[!htb]
\centering
 % 调整行间距
\scalebox{0.84}{
\begin{tabular}{lcccccccc}
\toprule
 & \multicolumn{2}{c}{\textbf{Pass Rate (\%)}} & \multicolumn{2}{c}{\textbf{Accuracy rate(\%)}} \\
\cmidrule(lr){2-3} \cmidrule(lr){4-5}
\textbf{} & \textbf{CodeContests} & \textbf{HumanEval} & \textbf{CodeContests} & \textbf{HumanEval} \\
\midrule
\textbf{HumanEval GPT-2} & & & & & & & & \\
\textbf{GPT-2} & 13.56 & 9.81  & 4.76 & 2.88  \\
\textbf{GPT-2-GPT4} & 54.72 & 39.41  & 26.84 & 19.17  \\
\textbf{GPT-2-GPT3.5} & 38.53 & 43.15  & 20.23 & 13.74  \\
\textbf{GPT-2-Llama} & 29.5 & 31.25  & 14.15 & 11.4  \\
\textbf{GPT-2-Wizard} & 38.7 & 30.46  & 12.7 & 9.06 \\
\midrule
\textbf{HumanEval GPT-Neo} & & & & & & & & \\
\textbf{GPT-Neo} & 14.48 & 10.75& 6.67 & 1.92 \\
\textbf{GPT-Neo-GPT4} & 44.44 & 49.18  & 26.24 & 24.44 \\
\textbf{GPT-Neo-GPT3.5} & 42.87 & 31.55  & 14.58& 9.98 \\
\textbf{GPT-Neo-Llama} & 40.27 & 32.39 & 13.25 & 10.55\\
\textbf{GPT-Neo-Wizard} & 33.72 & 29.86& 12.07 & 9.55\\
\bottomrule
\end{tabular}}
\caption{Result of "Better models help fine-tune normal models" experiment. On the top and bottom of the table, we show the performance of GPT-2 and GPT-Neo, and how they perform after they are fine-tuned by programs sampled by better models including GPT-4-turbo, GPT-3.5-turbo, CodeLlama-34B, WizardCoder-34B}
\label{table:accuracy}
\end{table*}
